# Supplementary material for: Pairing Tendencies in a Two-orbital Hubbard Model in One Dimension
Source: arXiv:1705.08780 source file (2017-07-02)
Supplement: Supplementary file 1 [file paper67_Supp.pdf]

# Supplementary Material for Pairing Tendencies in a Two-orbital Hubbard Model in One Dimension

N. D. Patel,[1,2] A. Nocera,[1,2] G. Alvarez,[3] A. Moreo,[1,2] and E. Dagotto[1,2]

[1]*Department of Physics and Astronomy, The University of Tennessee, Knoxville, Tennessee 37996, USA*
[2]*Materials Science and Technology Division, Oak Ridge National Laboratory, Oak Ridge, Tennessee 37831, USA*
[3]*Computer Science & Mathematics Division and Center for Nanophase Materials Sciences, Oak Ridge National Laboratory, Oak Ridge, Tennessee 37831, USA*

## I. USING DMRG++ WITH INPUTS

We use DMRG++ open source code for all the figures provided in the main text. One can download and run a quick test with DMRG++ by typing the following set of commands into a linux terminal (without the '$' sign).

```
$ cd someDirectory/
$ git clone https://github.com/g1257/PsimagLite.git
$ git clone https://github.com/g1257/dmrgpp.git
$ cd PsimagLite/lib
$ perl configure.pl
 (You may now edit Config.make)
$ make
$ cd ../../
$ cd dmrgpp/src
$ perl configure.pl
 (You may now edit Config.make)
$ make
$ ./dmrg -f ../TestSuite/inputs/input0.inp
$ ./toolboxdmrg -f ../TestSuite/inputs/input0.inp -a energies
```

Here, 'someDirectory' refers to the directory where you wish to download the files. After compilation, one can run the dmrg executable with inputs provided in an input file '`input0.inp`'. for this example, energy can be printed using the toolboxdmrg executable. One can use the provided input file (`L16_2OrbChain.inp`) to produce results for 16 sites two-orbital Hubbard chain at fixed $U/W = 1.60$ with fixed Hund coupling $J/U = 0.25$. The number of sites are specified with `TotalNumberOfSites=`, representing the total number of orbitals in the system. Interaction parameters for the given input file are

$$\begin{aligned} t &= -1.0 \\ U &= 1.60 \\ U' - J_H/2 &= 2.40 \\ -2J_H &= -3.20 \\ J_H &= 1.60 \end{aligned} \tag{1}$$

`SolverOptions=twositedmrg` is used to ask DMRG++ to use only two-site DMRG. The number of electrons can be specified using `TargetElectronsUp=`, `TargetElectronsDown=`. For example, one can use

```
TargetElectronsUp=16
TargetElectronsDown=16
```

to set 16 up and down electrons for a half-filled 16 sites two-orbital chain. Similarly, to reproduce results of two-hole doped system, one can use

```
TargetElectronsUp=15
TargetElectronsDown=15
```

Please refer to the DMRG++ user manual for information regarding the set up of finite and infinite system algorithm. Once the input file set up is completed, calculation of ground-state can be performed using

```
./dmrg -f L16_2OrbChain.inp
```

## II. CALCULATING OBSERVABLES

Once the ground state DMRG calculation is completed, real-space observables such as local occupation density (one-point), spin-spin correlations (ss), charge-charge correlations (nn), and pair-pair correlations (pp), can be calculated using the observe executable

```
./observe -f input2.inp onepoint,ss,nn,pp
```

One can also calculate other desired observables using the corresponding one-site operator. For example, one can calculate the double occupation by providing the $4 \times 4$ matrix for $n_\uparrow$ and $n_\downarrow$ (using a `nup.txt` and `ndn.txt` files) to the observe executable using

```
./observe -f input2.inp '<gs|:nup.txt;:ndn.txt|gs>'
```

where `nup.txt` is given by

```
TSPOperator=raw
RAW_MATRIX
4 4
0 0 0 0
0 0 0 0
0 0 1 0
0 0 0 1
FERMIONSIGN=1
JMVALUES 0 0
AngularFactor=1
```
